# Supplementary material for: Programming Unikernels in the Large via Functor Driven Development
Source: arXiv:1905.02529 source file (2019-05-07)
Supplement: Supplementary file 1 [file appendix.tex]

\clearpage
\pagestyle{empty}
\begin{SidewaysFigure}[1.05]
  \centering
  % Picture produced with the command:
  % dot -Tpng -Gdpi=150 -Gratio=compress -Gsize="25,30" mirage-www.dot
  \includegraphics[width=1.1\textheight]{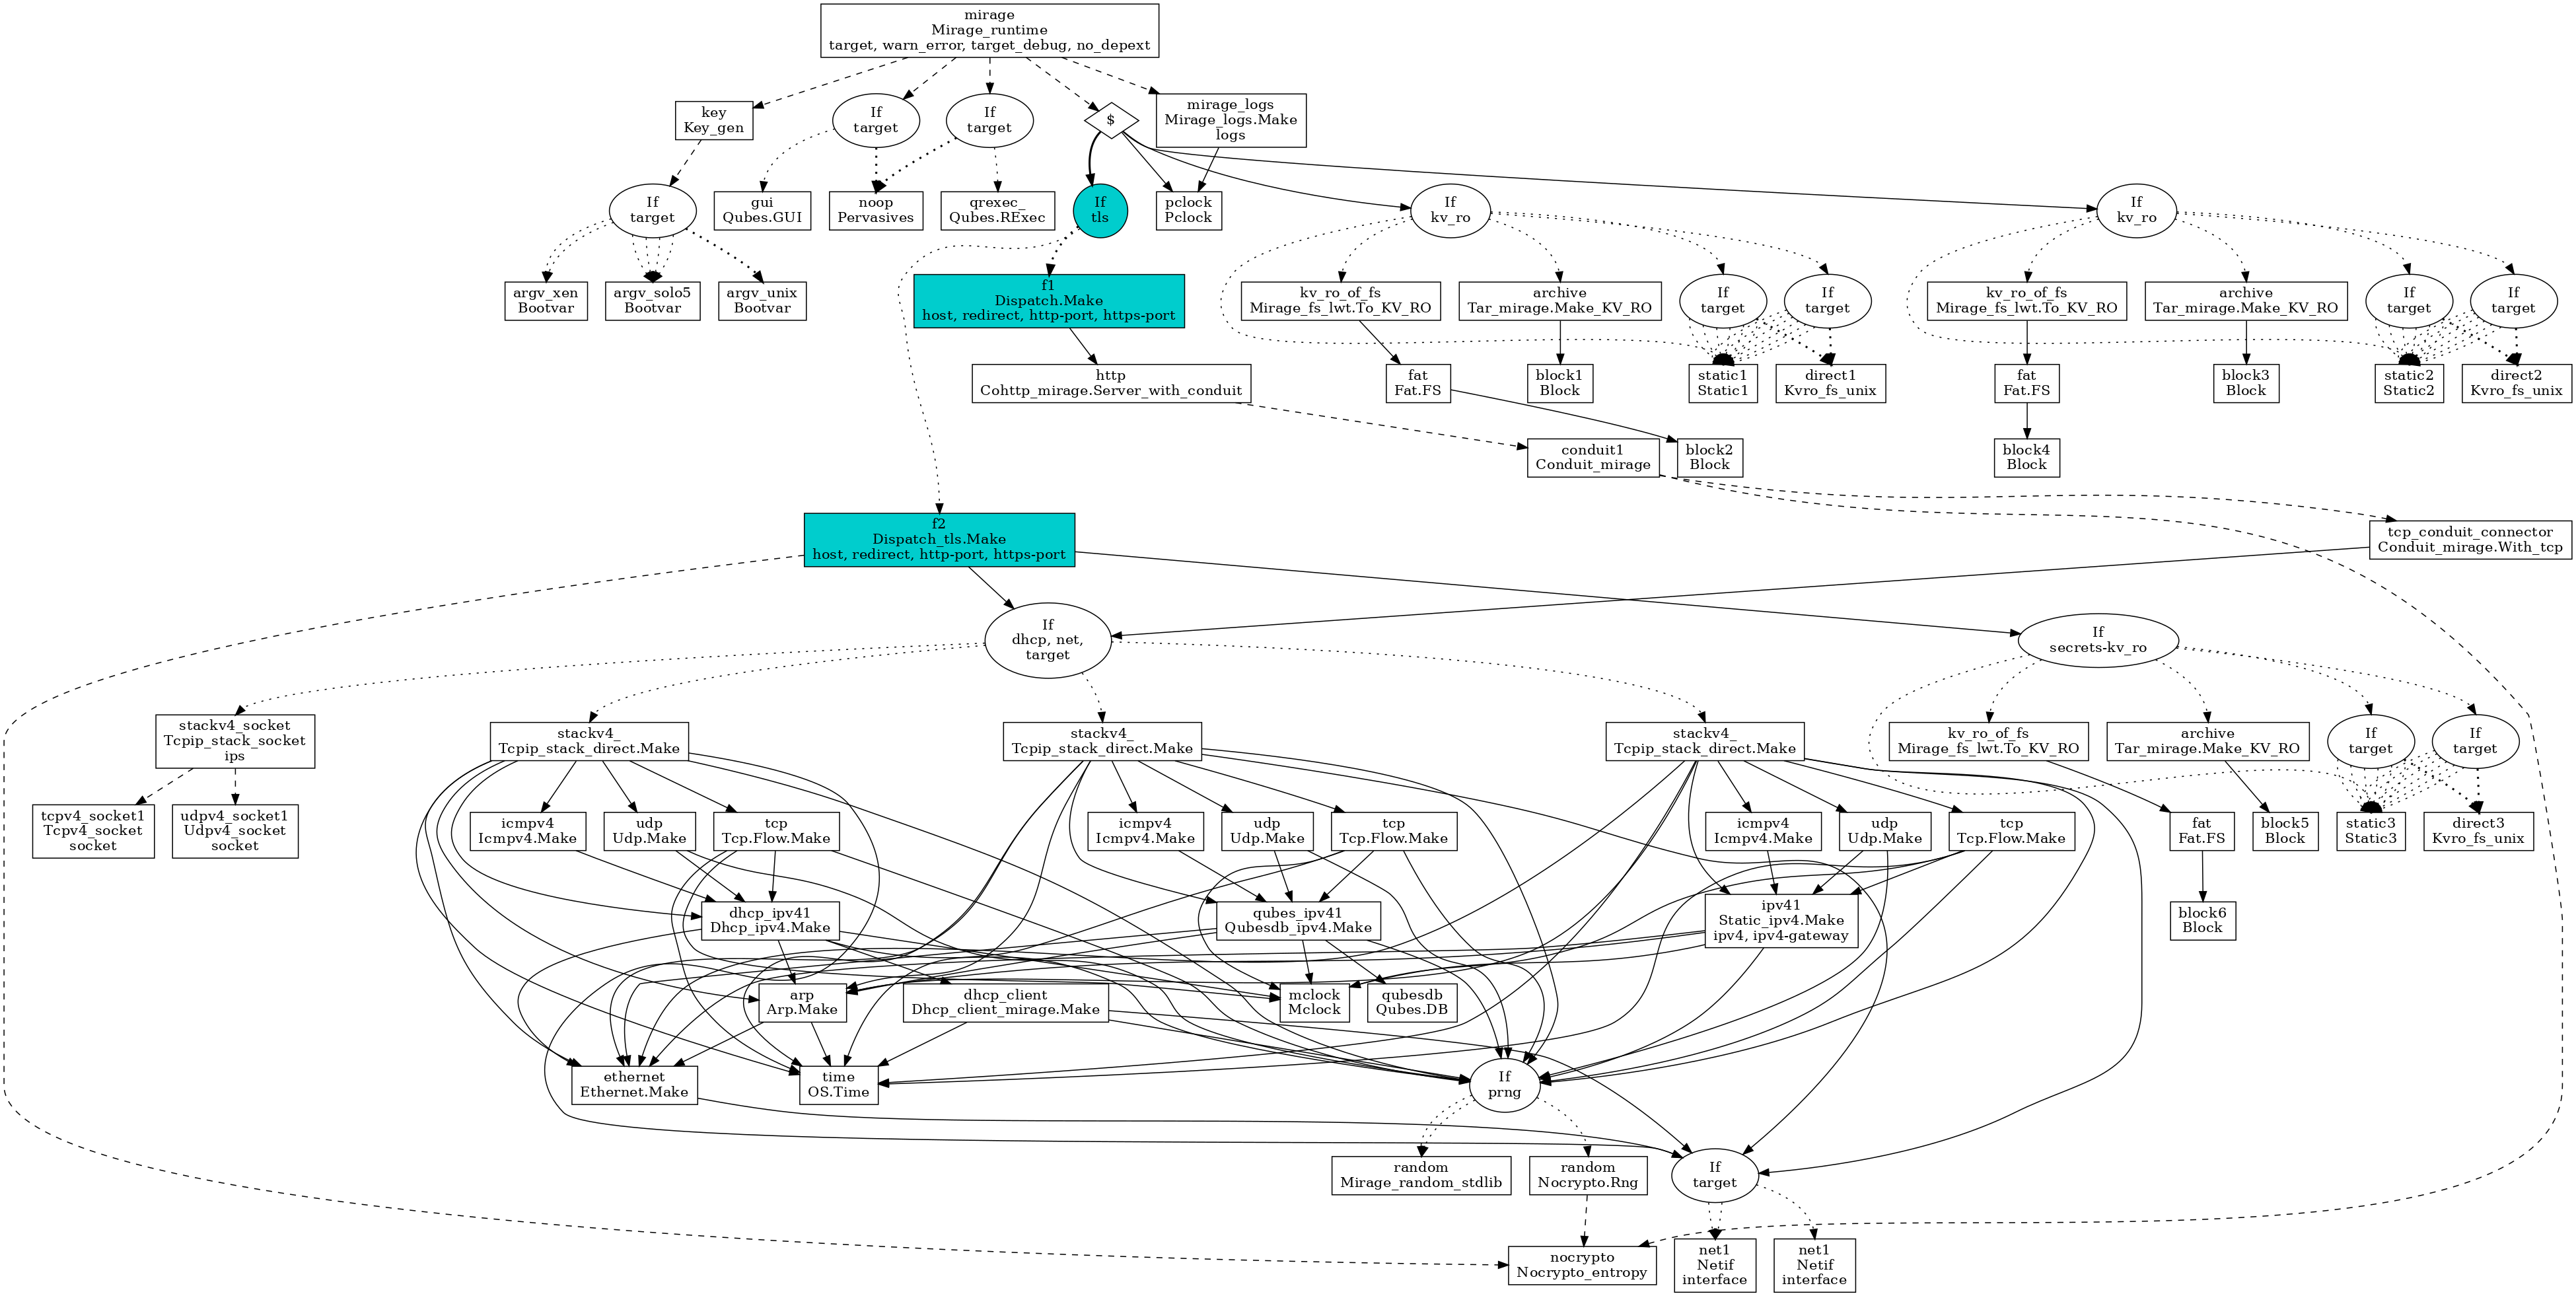}
  \caption{Architecture of the \mirage website -- \url{https://mirage.io/}}
  The devices and keys in colors are user-defined for the website. The rest
  is provided by the \mirage ecosystem.
  \label{website:dot}
\end{SidewaysFigure}
